# Supplementary material for: Design and Evaluation of IPFS: A Storage Layer for the Decentralized Web
Source: arXiv:2208.05877 source file (2022-08-11)
Supplement: Supplementary file 1 [file 10.appendix.tex]

\clearpage
\section{Appendix}

\begin{figure*}
    \centering
    \includegraphics[width=\textwidth]{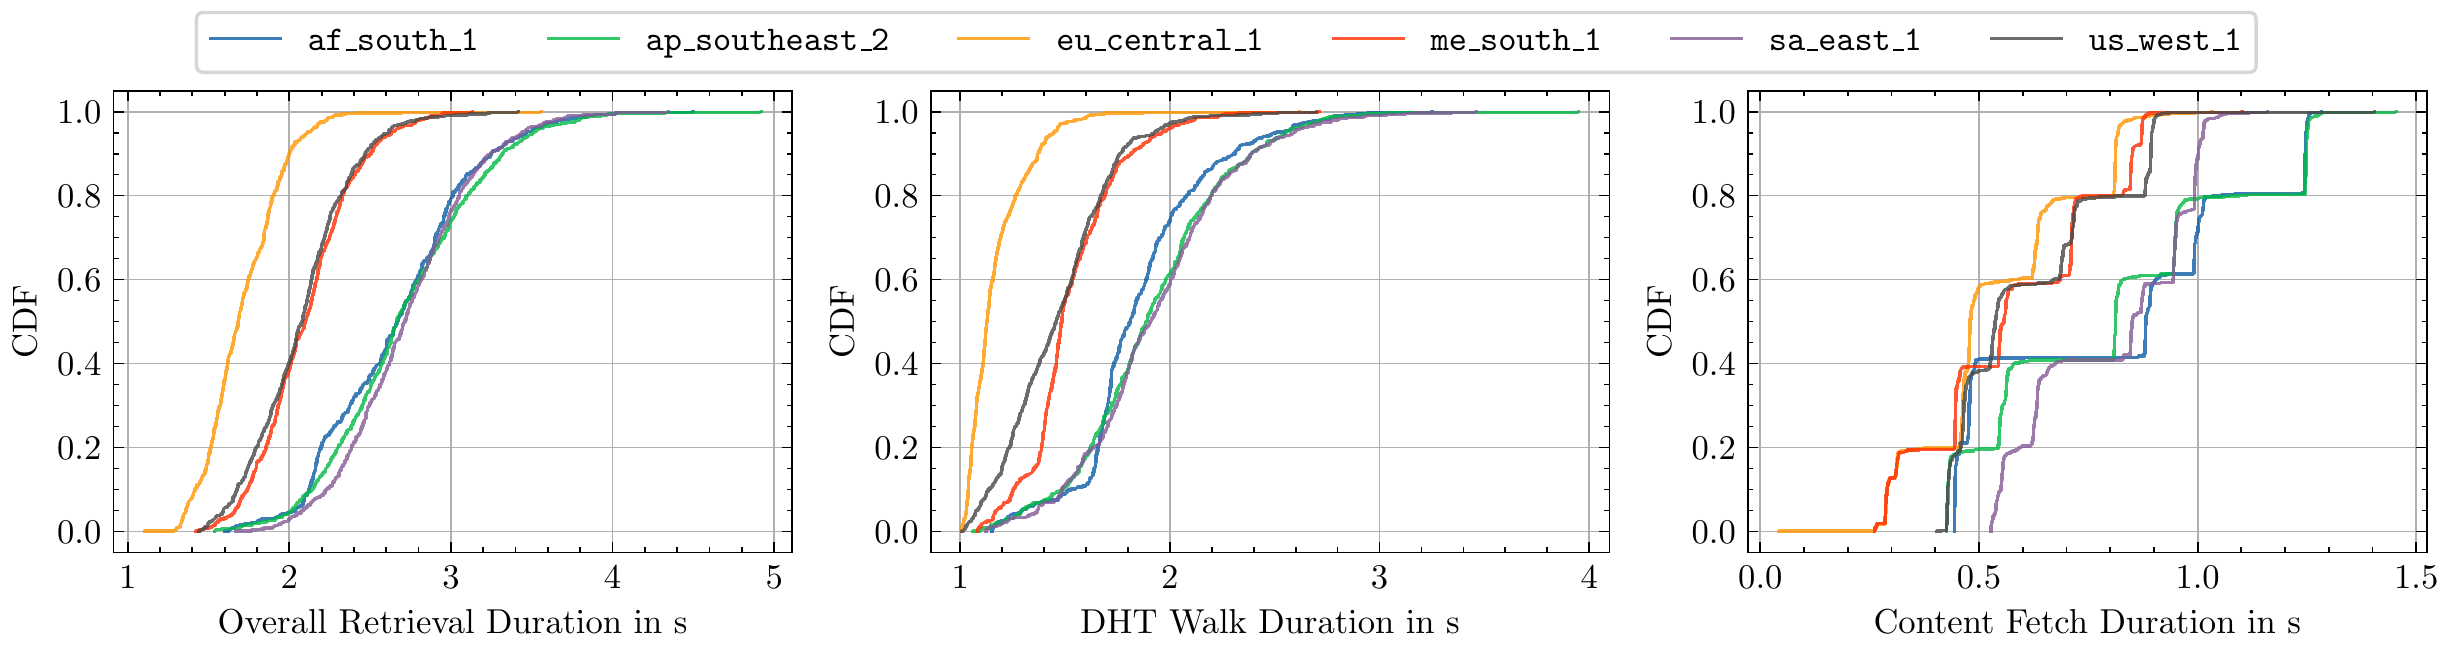}
    \caption{CDFs of the overall content retrieval operation (left), only the DHT walk to discover the providing peer (center) and content fetch duration (right). The right graph has a step shape due to the constant vantage points from where we are providing the content and the constant data size of the random data. The sample size is $4,324$ in all three graphs across all AWS regions combined.}
    \label{fig:dht_ret_process_combined}
\end{figure*}

\begin{figure*}
    \centering
    \includegraphics[width=\textwidth]{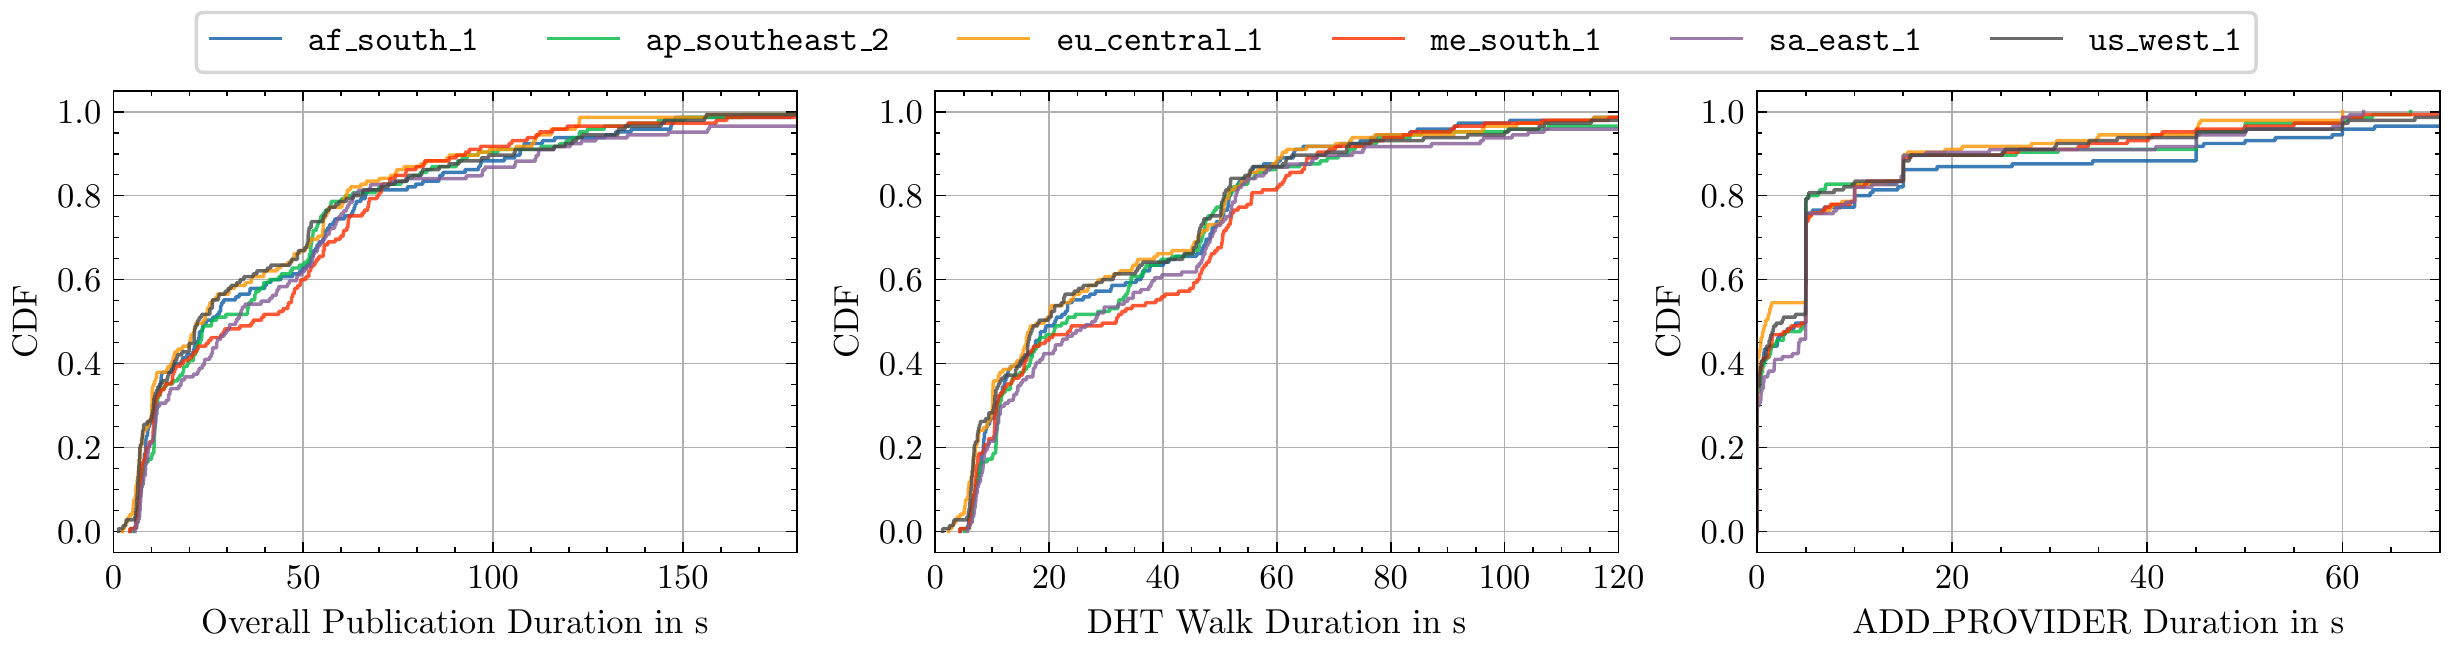}
    \caption{CDFs of the overall content publication operation (left), only the DHT walk to discover the appropriate peers to store the provider records (center) and the actual \texttt{ADD\_PROVIDER} RPC durations (right). The sample size is $869$ in all three graphs across all AWS regions combined.}
    \label{fig:dht_pvd_process_combined}
\end{figure*}

\begin{figure}
    \centering
    \includegraphics[width=\linewidth]{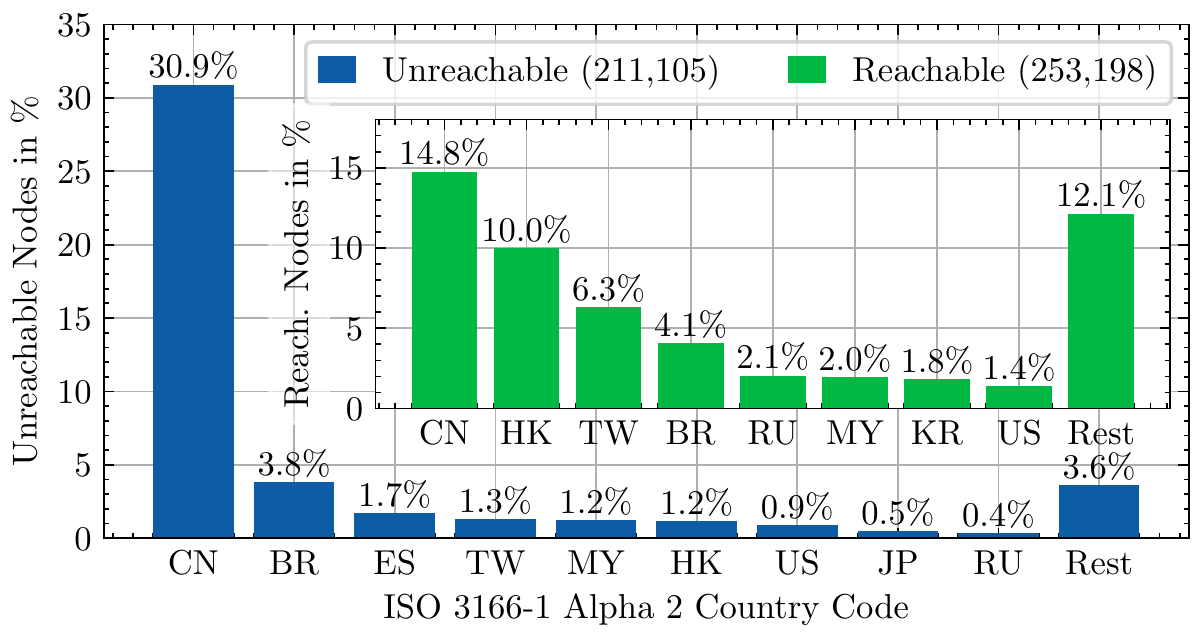} 
    \caption{Geographical distribution of IPFS nodes based on their IP addresses. Unreachable nodes correspond to nodes we were never able to connect to during the measurement period as opposed to reachable nodes which we were able to connect to at least once. The percentages are relative to the total number of $464,303$ observed unique IP addresses.}
    \label{fig:crawl_geo_nodes}
\end{figure}

\begin{figure}
    \centering
    \includegraphics[width=\linewidth]{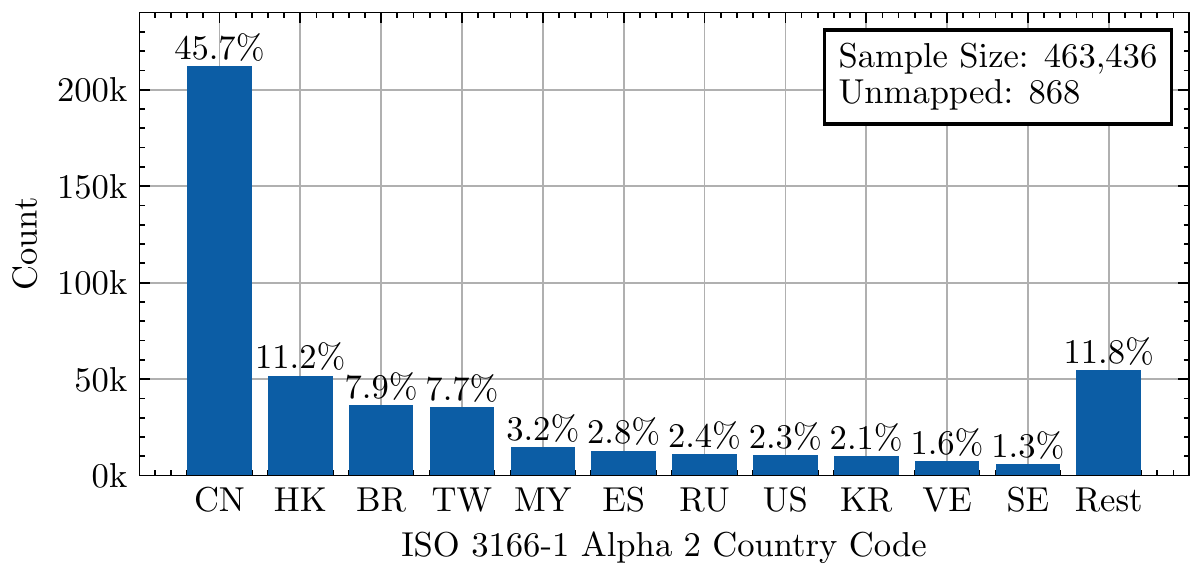} 
    \caption{Unique IP addresses found in the DHT from 2021-10-01 until 2021-11-01. In total $463,436$ unique addresses were found of which $868$ could not be mapped to a country. This may include IPv4 and IPv6 addresses of the same peer.}
    \label{fig:crawl_unique_ip_addresses}
\end{figure}

\begin{figure}
    \centering
    \includegraphics[width=\linewidth]{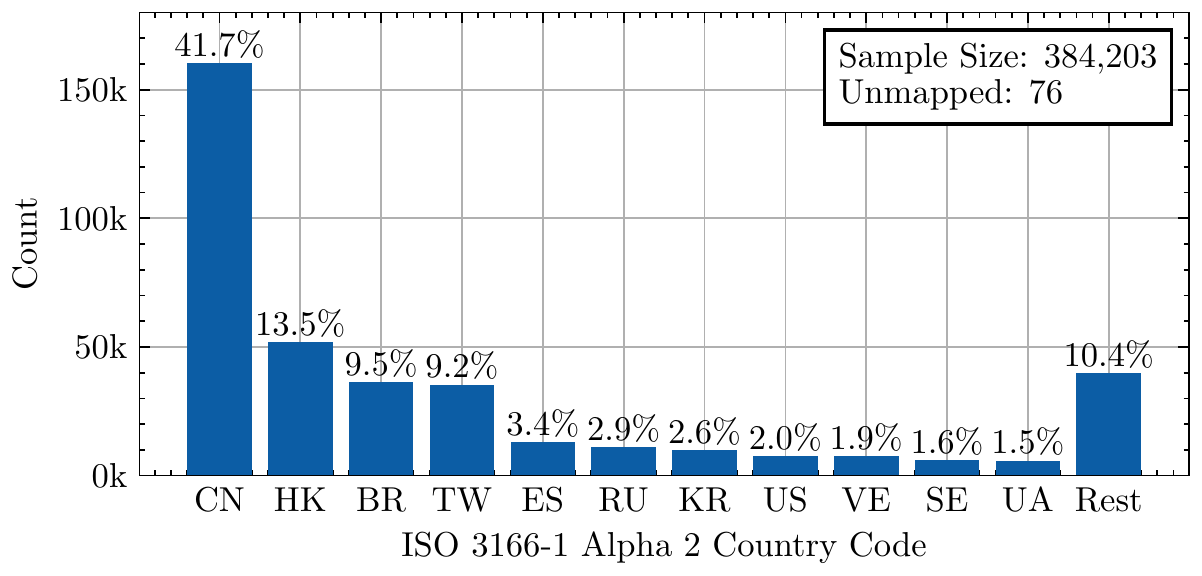} 
    \caption{Unique IPv4 addresses found in the DHT from 2021-10-01 until 2021-11-01. In total $384,203$ unique addresses were found of which $76$ could not be mapped to a country.}
    \label{fig:crawl_unique_ip_addresses_ipv4}
\end{figure}

\begin{figure}
    \centering
    \includegraphics[width=\linewidth]{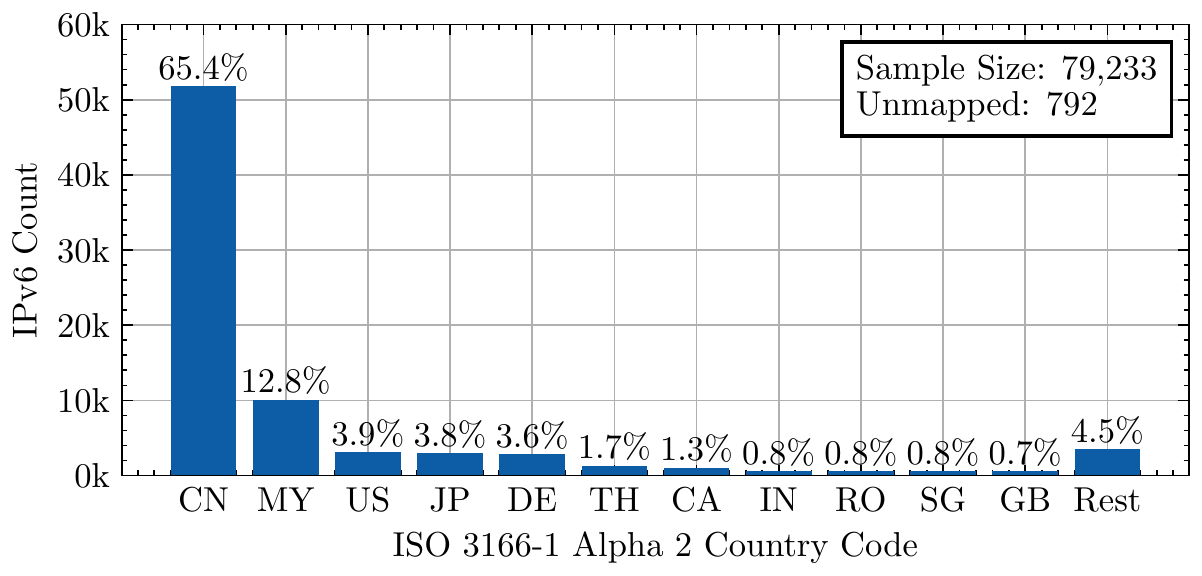} 
    \caption{Unique IPv6 addresses found in the DHT from 2021-10-01 until 2021-11-01. In total $79,233$ unique addresses were found of which $792$ could not be mapped to a country.}
    \label{fig:crawl_unique_ip_addresses_ipv6}
\end{figure}

\begin{figure}
    \centering
    \includegraphics[width=\linewidth]{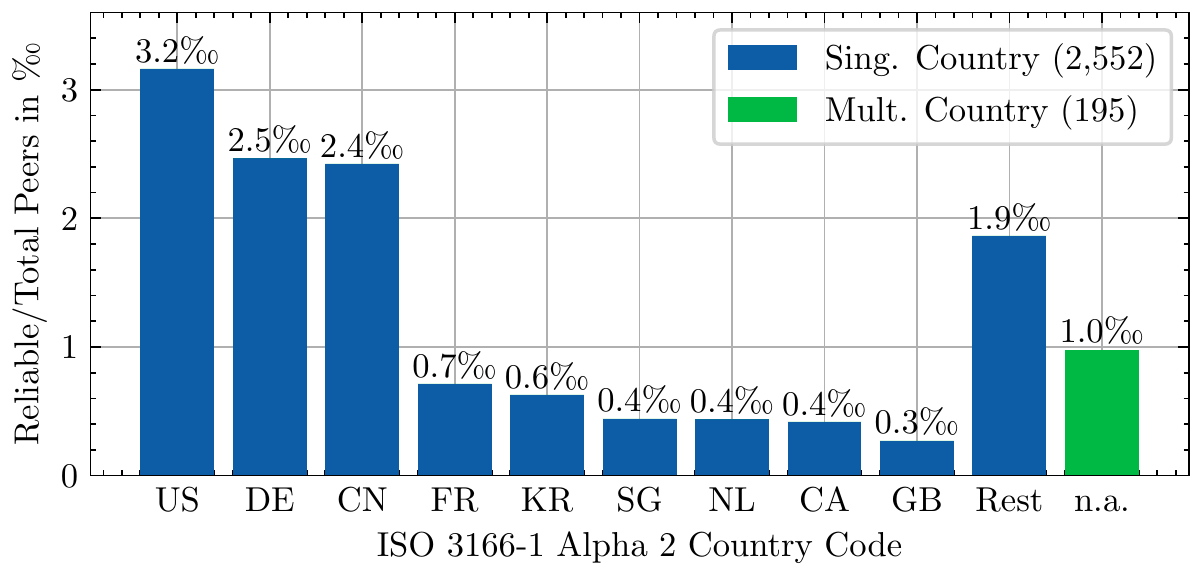} 
    \caption{Country distribution of reliable peers that were reachable for more than $90\%$ of the measurement period. Note the per mille as opposed to percent unit of the y-axis.}
    \label{fig:crawl_geo_reliable_peers}
\end{figure}

\begin{figure}
    \centering
    \includegraphics[width=\linewidth]{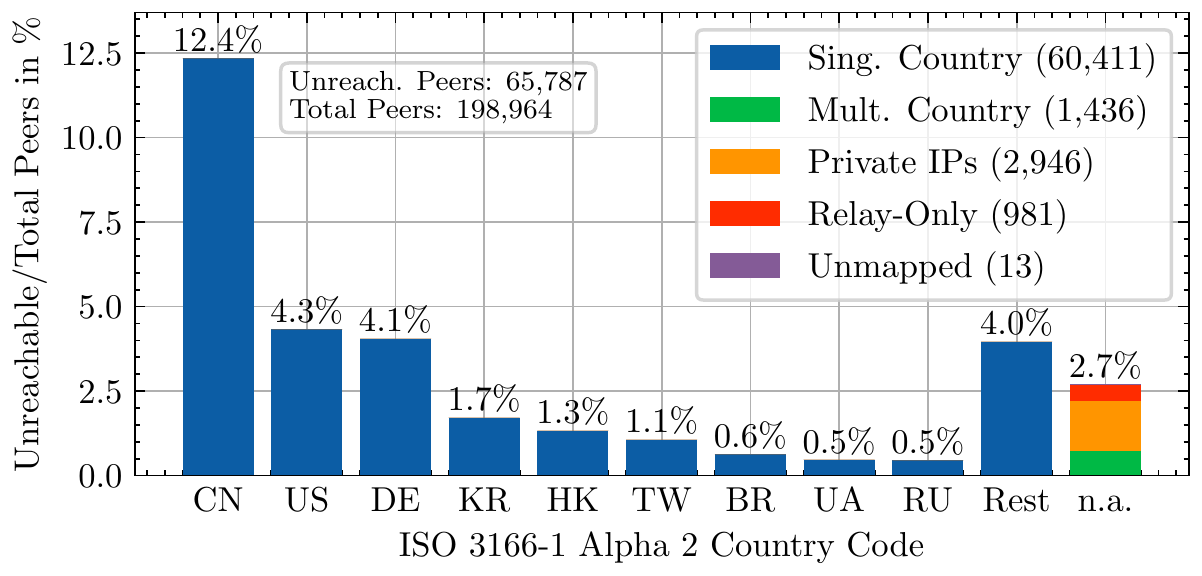} 
    \caption{Country distribution of unreachable peers. ``Unmapped'' includes peers that only provided DNS multi addresses that could not be resolved to an IP address and IP addresses that were not found in the GeoIP database.}
    \label{fig:crawl_geo_offline_peers}
\end{figure}
