# Supplementary material for: Design and Evaluation of IPFS: A Storage Layer for the Decentralized Web
Source: arXiv:2208.05877 source file (2022-08-11)
Supplement: Supplementary file 2 [file 11.appendix-git.tex]

% \clearpage
\section{Appendix}

%%%%%%%%%%%%%%%%%%%%%%%%%%%%%%%%%%%%%%%%%%%%%%%%%%%%%%%%%%%%%%%%%%%%%%%%%%%%%%%
\subsection{Development Data}
\label{sec:evaluation_git}
%%%%%%%%%%%%%%%%%%%%%%%%%%%%%%%%%%%%%%%%%%%%%%%%%%%%%%%%%%%%%%%%%%%%%%%%%%%%%%%

The source code of IPFS is publicly available in Github~\cite{ipfs-git} allowing anyone to clone and contribute. In fact, an isolated ecosystem of IPFS instances has been implemented and used by platforms such as D-tube~\cite{dtube} for decentralised video streaming and Filecoin~\cite{fc-ipfs} for blockchain-based storage. In this section, we briefly summarise and describe the development efforts of the main IPFS  repositories.

\begin{table*}[htbp]
\centering
\caption{Details of repositories in IPFS and their description}
\resizebox{1\linewidth}{!}{
\begin{tabular}{llrrrrlrl} 
\toprule
name           & created at                & \begin{tabular}[c]{@{}r@{}}\#contributors\\(PL\%)\end{tabular} & \#commits & \#forks                   & \#stars                   & language & \begin{tabular}[c]{@{}r@{}}Size\\(MB)\end{tabular} & Description                                                                                                                          \\ 
\midrule
go-ipfs        & 2014-06-26                & 301                                                       & 12659     & 2466                      & 12787                     & Go       & 44.1                                               & IPFS implementation in Go                                                                                                            \\
js-ipfs        & 2014-05-30                & 230                                                       & 6313      & 1193                      & 6304                      & JS       & 54.5                                               & IPFS implementation in JS                                                                                                            \\
ipfs-cluster   & 2016-07-01                & 35                                                        & 2453      & 208                       & 1100                      & Go       & 12.7                                               & Pinset orchestration for IPFS                                                                                                        \\
ipfs-docs      & 2019-10-23                & 125                                                       & 2272      & 220                       & 161                       & Go       & 55.5                                               & IPFS documentation platform                                                                                                          \\
ipfs-companion & 2015-03-22                & 36                                                        & 1680      & 270                       & 1587                      & JS       & 11.3                                               & \begin{tabular}[c]{@{}l@{}}Browser extension to access\\resources on the IPFS\end{tabular}                     \\
ipfs-blog      & 2020-12-03                & 24                                                        & 1399      & 9                         & 21                        & Vue      & 341.7                                              & IPFS Blog  News                                                                                                                      \\
go-bitswap     & 2018-07-27                & 45                                                        & 1340      & 74                        & 170                       & Go       & 3.2                                                & \begin{tabular}[c]{@{}l@{}}The golang implementation \\of the bitswap protocol\end{tabular}                                          \\
team-mgmt      & 2015-03-29                & 77                                                        & 1306      & 109                       & 255                       & JS       & 6.7                                                & \begin{tabular}[c]{@{}l@{}}IPFS Team Planning, \\Management~Coordination threads\end{tabular}                                             \\
ipfs-webui     & 2014-09-26                & 74                                                        & 1232      & 398                       & 1190                      & JS       & 36.6                                               & A frontend for an IPFS node.                                                                                                         \\
ipfs-desktop   & 2015-05-30                & 41                                                        & 1207      & 612                       & 3848                      & JS       & 16.8                                               & \begin{tabular}[c]{@{}l@{}}Desktop application for IPFS on \\Windows, Mac and Linux.\end{tabular}  \\ 
\hline
\multicolumn{2}{c}{All 177 repositories}   & 1185 (3.6\%)                                                    & 60415  (62.26\%)      & \multicolumn{1}{l}{10383} & \multicolumn{1}{l}{58778} &          & \multicolumn{1}{l}{1398.3}                         &                                                                                                                                      \\
\bottomrule
\end{tabular}
}
\label{tab:git_ipfs_summary}
\end{table*}

We capture the development statistics for the repositories using gihub APIs~\cite{api-git}. The IPFS project hosts 177 public repositories, with a total of 1.18K code contributors. Table~\ref{tab:git_ipfs_summary} presents the summary of top ten repositories based on number of commits to the repositories. Major activities can be seen in Go~\cite{go-ipfs-git} (\texttt{go-ipfs}) and Javascript~\cite{js-ipfs-git} (\texttt{js-ipfs}) variants representing the core development, with both the repositories being created around the same time and being actively developed for 6 years. Figure~\ref{fig:git_ipfsjsgo_plot} shows the development timeline through line additions, deletions and the files changed. Looking at \texttt{go-ipfs}, we see contributions soaring between 2015 and 2017, while similar trends for \texttt{js-ipfs} are observed from April 2019 onwards. 
% Looking at \texttt{js-ipfs}, we see contributions soaring from April 2019, when \texttt{go-ipfs} stabilized in terms of codebase contributions.
Interestingly, we notice that only 8.8\% of common contributors between the two repositories showing interest from the community to develop and deploy variants in other programming languages. There are also recent development efforts in other programming languages (\eg rust~\cite{rust-ipfs-git} , python~\cite{python-ipfs-git}) by other users/organisations following the underlying specifications~\cite{ipfs-specs-git}. 

Further, core components of IPFS such as libp2p~\cite{libp2p-impls}, IPLD~\cite{ipld-git} have evolved into different projects with only less than 1\% of contributors common between any combination of these components with Go and Javascript variants, showing good participation from different users in the community, yet the components being interoperable.

% The source code of IPFS is publicly available in Github~\cite{} for anyone to clone and contribute. In fact, isolated ecosystem of IPFS instances have been implemented and used by platforms such as D-tube~\cite{} for decentralised video streaming and Filecoin for blockchain based storage. In this section, we summarise and describe the development efforts of the main IPFS  repositories. 

% The IPFS hosts 177 public repositories, with a total of 1.18K contributors. 

% Also, there exist variants of IPFS in terms of programming languages (\eg rust~\cite{}, python~\cite{}) developed by different users/organisations but following the technical protocol specifications in XX.

% https://github.com/rs-ipfs/rust-ipfs https://github.com/ipfs-shipyard/py-ipfs 

% Peers in the IPFS network follow a set of technical protocol specifications\footnote{SHA1: \texttt{\shaSpecs} -- \url{https://github.com/ipfs/specs}} of which there exist one reference implementation written in Go and two implementations in alpha state written in JavaScript and Rust. The results shown below were gathered directly from their respective git repositories go-ipfs\footnote{SHA1: \texttt{\shaGoIPFS} -- \url{https://github.com/ipfs/go-ipfs}}, js-ipfs\footnote{SHA1: \texttt{\shaJsIPFS} -- \url{https://github.com/ipfs/js-ipfs}} and rust-ipfs\footnote{SHA1: \texttt{\shaRustIPFS} -- \url{https://github.com/rs-ipfs/rust-ipfs}} and were collected on the 9th of December 2021.
% \usepackage{booktabs}

% \usepackage{booktabs}
\begin{figure}
    \centering
    \includegraphics[width=\linewidth]{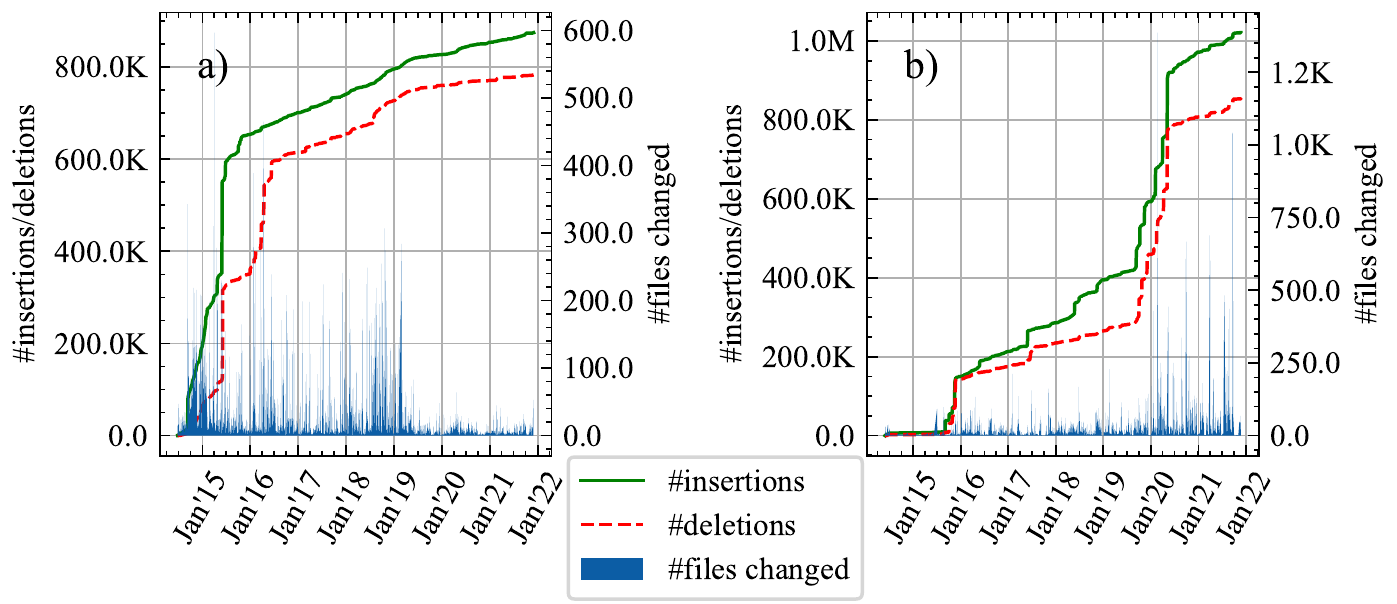} 
    \caption{Development activities of IPFS variants a) Go Implementation b) JS Implementation}
    \label{fig:git_ipfsjsgo_plot}
\end{figure}
